# Supplementary material for: Revisiting Reciprocal Recommender Systems: Metrics, Formulation, and Method
Source: arXiv:2408.09748 source file (2024-08-19)
Supplement: Supplementary file 1 [file sec_appendix.tex]

% \newpage

% The algorithm of our proposed CRRS is summarized in \autoref{algo:crrs}.

\section{Iterative calculation method for proposed metrics}

In this section, we conduct a discussion to analyze the computational cost for calculating the proposed metrics and propose a refined iterative method to enable real-time updating.

The calculation of all the proposed metrics requires that all users' recommendation lists have been confirmed. 
Consequently, it can not be calculated with each training batch.
For instance,  given a user from $\mathcal{A}$, we need to compute the preference score from each user from $\mathcal{B}$ to determine the redundant recommendations. 
This computation process is highly time-consuming and involves an exponential number of predictions.  
%For instance, in calculating CRecall for a top-20 recommendation, if five positive matches are recalled for an $A$-side user $a_i$, it becomes necessary to generate recommendation lists for these five $B$-side users and verify whether $a_i$ is included in them. 
%This process involves an exponential number of predictive tasks, especially for real-world scenarios with large-scale data.

To enable efficient updating of the proposed metrics concurrent with the training process, we design an iterative method that  
 requires only the recording of a modifiable set of positive pairs, denoted as $\mathcal{P} = \{(a_i, b_j) | r_{ij} = 1\}$.
Given the current metrics $\mathrm{CRecall}^{(t)}$ and $\mathrm{CPrecision}^{(t)}$,
a new prediction is completed with the number of true positive samples denoted as $\mathrm{TP}^{(t+1)}$ and the total number of this user's positive instances as $\mathrm{M}^{(t+1)}$, regardless of the user's side.
To commence the iterative process, we first calculate the overlap between its positive samples and the set~$\mathcal{P}$, denoted as $\mathrm{RM}^{(t+1)}$, representing the count of redundant recommendations brought by this user. Subsequently, the metrics can be updated using the following iterative formula:
\begin{align}
    \mathrm{CRecall}^{(t+1)} &= \frac{\mathrm{CRecall}^{(t)} \cdot |\mathcal{P}| + \mathrm{TP}^{(t+1)} - \mathrm{RM}^{(t+1)}}{|\mathcal{P}| + \mathrm{M}^{(t+1)} - \mathrm{RM}^{(t+1)}}, \\
    \mathrm{CPrecision}^{(t+1)} &= \frac{\mathrm{CPrecision}^{(t)} \cdot t  K + \mathrm{TP}^{(t+1)} - \mathrm{RM}^{(t+1)}}{(t + 1) K}, \\
    \mathrm{SRecall}^{(t+1)} &= \frac{\mathrm{SRecall}^{(t)} \cdot |\mathcal{P}| + \mathrm{RM}^{(t+1)}}{|\mathcal{P}| + \mathrm{M}^{(t+1)} - \mathrm{RM}^{(t+1)}}, \\
    \mathrm{SPrecision}^{(t+1)} &= \frac{\mathrm{SPrecision}^{(t)} \cdot t  K + \mathrm{RM}^{(t+1)}}{(t + 1)  K},
\end{align}
where $K$ is the length of the recommendation list for each user.

As such, the proposed metrics for overall coverage and bilateral stability can be updated in real time.
This approach significantly enhances the system's efficiency, making it scalable for large-scale and dynamic real-world scenarios.
